# Supplementary material for: 13CFLUX -- Third-generation high-performance engine for isotopically (non)stationary 13C metabolic flux analysis
Source: arXiv:2509.23847 source file (2025-09-28)
Supplement: Supplementary file 1 [file simulator_table.pdf]

|                 | Publication Date | Global (flux map) vs. Local (flux ratios) | State space |         |     | Simulation |      | Measurements |           |     | Workflows         |                      | Availability         |                       |                         |           |                              |                                                                                                                                                                                                                        |
|-----------------|------------------|-------------------------------------------|-------------|---------|-----|------------|------|--------------|-----------|-----|-------------------|----------------------|----------------------|-----------------------|-------------------------|-----------|------------------------------|------------------------------------------------------------------------------------------------------------------------------------------------------------------------------------------------------------------------|
|                 |                  |                                           | Isotopomer  | Cumomer | EMU | IST        | INST | MS           | Tandem-MS | NMR | Parameter fitting | Statistical analysis | Design of experiment | Platform independence | Commercial dependencies | Open code | License                      | Reference                                                                                                                                                                                                              |
| tcaSIM, tcaCALC | 1996             | L                                         | X           |         |     | X          |      | X            |           | X   | X                 | FS                   |                      |                       |                         |           | ?                            | <a href="https://doi.org/10.1002/mrm.1910360318">https://doi.org/10.1002/mrm.1910360318</a><br><a href="https://invivometabolism.org/tca.html">https://invivometabolism.org/tca.html</a>                               |
| 13C-FLUX        | 2001             | G                                         | X           |         |     | X          |      | X            |           | X   | X                 | FS                   | X                    |                       |                         |           | custom (academic/commercial) | <a href="https://doi.org/10.1006/mben.2001.0188">https://doi.org/10.1006/mben.2001.0188</a><br><a href="https://13cflux.net/13cflux">https://13cflux.net/13cflux</a>                                                   |
| 13CFLUX2        | 2013             | G                                         |             | X       | X   | X          |      | X            | X         | X   | X                 | FS, PB, PL           | X                    |                       |                         |           | custom (academic/commercial) | <a href="https://doi.org/10.1093/bioinformatics/bts646">https://doi.org/10.1093/bioinformatics/bts646</a><br><a href="https://13cflux.net/13cflux2">https://13cflux.net/13cflux2</a>                                   |
| 13CFLUXv3       | 2025             | G                                         |             | X       | X   | X          | X    | X            | X         | X   | X                 | FS, PB, PL, MCMC     | X                    | X                     |                         | X         | AGPL                         | <a href="https://13cflux.net/13cflux3">https://13cflux.net/13cflux3</a>                                                                                                                                                |
| FiatFlux        | 2005             | L                                         |             |         |     | X          |      | X            |           |     | X                 | FS                   |                      | X                     | MATLAB                  |           | custom (academic/commercial) | <a href="https://doi.org/10.1186/1471-2105-6-209">https://doi.org/10.1186/1471-2105-6-209</a>                                                                                                                          |
| SUMO FLUX       | 2016             | L                                         |             |         |     | X          |      | X            | X         |     | X                 | PB                   |                      | X                     | MATLAB                  | X         | GPLv3                        | <a href="https://doi.org/10.1371/journal.pcbi.1005109">https://doi.org/10.1371/journal.pcbi.1005109</a><br><a href="https://github.com/zamboni-lab/sumoflux">https://github.com/zamboni-lab/sumoflux</a>               |
| METRAN          | 2008             | G                                         |             |         | X   | X          |      | X            |           |     | X                 | PL                   | X                    | X                     |                         |           | ?                            | <a href="https://doi.org/10.1074/jbc.M706494200">https://doi.org/10.1074/jbc.M706494200</a><br><a href="https://cheresearch.engin.umich.edu/mranton/metrans/">https://cheresearch.engin.umich.edu/mranton/metrans/</a> |
| OpenFlux        | 2009             | G                                         |             |         | X   | X          |      | X            |           |     | X                 | PB, PL               | X                    | X                     | MATLAB                  | X         | GPLv2                        | <a href="https://doi.org/10.1186/1475-2859-8-25">https://doi.org/10.1186/1475-2859-8-25</a><br><a href="https://sourceforge.net/projects/openflux">https://sourceforge.net/projects/openflux</a>                       |
| influx_s        | 2012             | G                                         |             | X       | X   | X          |      | X            |           | X   | X                 | FS, PB               |                      | X                     |                         | X         | GPLv2                        | <a href="https://doi.org/10.1093/bioinformatics/btr716">https://doi.org/10.1093/bioinformatics/btr716</a><br><a href="https://github.com/sgsokol/influx">https://github.com/sgsokol/influx</a>                         |
| influx_si       | 2021             | G                                         |             | X       | X   |            | X    | X            |           | X   | X                 | FS, PB               |                      | X                     |                         | X         | GPLv2                        | <a href="https://doi.org/10.1128/AEM.00719-21">https://doi.org/10.1128/AEM.00719-21</a><br><a href="https://github.com/sgsokol/influx">https://github.com/sgsokol/influx</a>                                           |
| INCA            | 2014             | G                                         |             |         | X   | X          | X    | X            |           | 1H  | X                 | FS, PB, PL           | X                    | X                     | MATLAB                  |           | custom (academic/commercial) | <a href="https://doi.org/10.1093/bioinformatics/btu015">https://doi.org/10.1093/bioinformatics/btu015</a><br><a href="https://mfa.vueinnovations.com">https://mfa.vueinnovations.com</a>                               |
| INCA2           | 2022             | G                                         |             |         | X   | X          | X    | X            |           | X   | X                 | FS, PB, PL           | X                    | X                     | MATLAB                  |           | custom (academic/commercial) | <a href="https://doi.org/10.1016/j.jymben.2021.12.009">https://doi.org/10.1016/j.jymben.2021.12.009</a><br><a href="https://mfa.vueinnovations.com">https://mfa.vueinnovations.com</a>                                 |
| Open Mebius     | 2014             | G                                         |             |         | X   | X          | X    | X            |           |     | X                 | PL                   |                      |                       | MATLAB                  | X         | ?                            | <a href="https://doi.org/10.1155/2014/627014">https://doi.org/10.1155/2014/627014</a><br><a href="https://en.metabolic-engineering.jp/page/software">https://en.metabolic-engineering.jp/page/software</a>             |
| mfapy           | 2021             | G                                         |             |         | X   | X          | X    | X            |           |     | X                 | PL                   | X                    | X                     |                         | X         | MIT                          | <a href="https://doi.org/10.1016/j.mec.2021.e00177">https://doi.org/10.1016/j.mec.2021.e00177</a><br><a href="https://github.com/tumiomatsuda/mfapy">https://github.com/tumiomatsuda/mfapy</a>                         |
| OpenFlux2       | 2014             | G                                         |             |         | X   | X          |      | X            |           |     | X                 | FS, PB, PL           | X                    | X                     | MATLAB                  | X         | GPLv2                        | <a href="https://doi.org/10.1186/s12934-014-0152-x">https://doi.org/10.1186/s12934-014-0152-x</a><br><a href="https://sourceforge.net/projects/openflux2">https://sourceforge.net/projects/openflux2</a>               |
| sysmetab        | 2016             | G                                         |             | X       |     | X          | X    | X            |           | X   | X                 | FS, PB               |                      | X                     |                         |           | ?                            | <a href="https://doi.org/10.1109/TCBB.2016.2544299">https://doi.org/10.1109/TCBB.2016.2544299</a><br><a href="https://gitlab.com/scilab/forge/sysmetab/">https://gitlab.com/scilab/forge/sysmetab/</a>                 |
| WUFlux          | 2016             | G                                         |             |         | X   | X          |      | X            |           |     | X                 | PB                   |                      | X                     | MATLAB                  | X         | ?                            | <a href="https://doi.org/10.1186/s12859-016-1314-0">https://doi.org/10.1186/s12859-016-1314-0</a><br><a href="https://tang.eece.wustl.edu/ToolDevelopment.htm">https://tang.eece.wustl.edu/ToolDevelopment.htm</a>     |
| FluxPyt         | 2018             | G                                         |             |         | X   | X          |      | X            |           |     | X                 | PB                   |                      | X                     |                         | X         | BSD-3                        | <a href="https://doi.org/10.7717/peerj.4716">https://doi.org/10.7717/peerj.4716</a><br><a href="https://sourceforge.net/projects/fluxpyt">https://sourceforge.net/projects/fluxpyt</a>                                 |
| EMUlator        | 2019             | G                                         |             |         | X   | X          |      | X            |           |     |                   | none                 |                      |                       |                         |           | ?                            | <a href="https://doi.org/10.3389/fmicb.2019.00922">https://doi.org/10.3389/fmicb.2019.00922</a>                                                                                                                        |
| freeflux        | 2023             | G                                         |             |         | X   | X          | X    | X            |           |     | X                 | PB                   |                      | X                     |                         | X         | GPLv3                        | <a href="https://doi.org/10.1021/acssynbio.3c00265">https://doi.org/10.1021/acssynbio.3c00265</a><br><a href="https://github.com/Chaowu88/freeflux">https://github.com/Chaowu88/freeflux</a>                           |
| eiFlux          | 2022             | G                                         |             | X       | X   | X          | X    | X            | X         |     | X                 | PB                   |                      | X                     | GAMS                    |           | ?                            | <a href="https://doi.org/10.1371/journal.pcbi.1009831">https://doi.org/10.1371/journal.pcbi.1009831</a>                                                                                                                |
| CeCaFlux        | 2022             | G                                         |             |         | X   | X          | X    | X            |           |     | X                 | PL                   |                      | X                     |                         |           | ?                            | <a href="https://doi.org/10.1093/bioinformatics/btac341">https://doi.org/10.1093/bioinformatics/btac341</a><br><a href="https://github.com/zhzhd82/CeCaFLUX">https://github.com/zhzhd82/CeCaFLUX</a>                   |
| BayFlux         | 2024             | G                                         |             |         | X   | X          |      | X            |           |     |                   | MCMC                 |                      | X                     |                         | X         | custom (free usage)          | <a href="https://doi.org/10.1371/journal.pcbi.1011111">https://doi.org/10.1371/journal.pcbi.1011111</a><br><a href="https://github.com/JBEI/bayflux">https://github.com/JBEI/bayflux</a>                               |

etran.html

e/openmebius

ml
